# Supplementary material for: KG-ECO: Knowledge Graph Enhanced Entity Correction for Query Rewriting
Source: arXiv:2302.10454 source file (2023-02-22)
Supplement: Supplementary file 1 [file appendix_bck.tex]

%%%%%%%%%%%%%%%%%%%%%%%%%%%%%%%%%%%%%%%%%%%%%
% \newpage

\appendix

\section{Appendix}
\label{sec: appendix}

%%%%%%%%%%%%%%%%%%%%%%%%%%%%%%%%%%%%%%%%%%%%%
\subsection{Experimental Setup}
\label{subsection: Experimental Setup}
In both L1 and L2 layers, we utilize RoBERTa-BASE model (110M parameters). The GAT encoder has $4$ layers with $8$ attention heads and hidden dimension = $400$. We do not apply dropout in GAT layers.  

All training experiments are conducted end-to-end: we train RoBERTa and GAT simultaneously. We use  Adam optimizer with linear decay of learning rate. All the experiments are performed with NVIDIA Tesla V100 GPUs in a single run. For L1 training: Initial learning rate = $8e-4$. Batch size = $64$. Number of training epochs = $10$. Training takes $\sim 40$ GPU hours. For L2 training: Initial learning rate = $5e-4$. Batch size = $32$. Number of training epochs = $4$. Training takes $\sim 70$ GPU hours.  

Hard negative entity samples are obtained from top K incorrect predictions of L1 retrieval model, which is fine-tuned on training data, without using any KG information. In L1 training, we use 1 hard negative for each sample, while in L2 training, we use 4 hard negatives for each sample.

\subsection{Future Work: Combining Entity Level and Utterance Level Approaches}
One limitation of our approach is that it only corrects entity corruption. For instance, consider the utterance pair: ``volume two twenty five percent'' and ``volume to twenty five percent''. The source utterance contains a friction, but there is no entity. In this case, the entity correction system cannot produce desired rewrite.

For future work, we will consider combining our entity correction system with utterance level QR system. A possible design is the following: We utilize entity correction system as the first priority. If the entity correction is not triggered, then we turn to the second priority, the utterance level QR system. This way we can handle both of the following two scenarios: (1) An entity corruption exists. It’s reasonable to prioritize entity correction system, as it has superior performance on friction set. (2) No entity corruption exists. Most likely the entity correction system will not be triggered, as a null span would be predicted. However, there may still be some non-entity friction, which can be corrected by the utterance level QR system.
